# Supplementary material for: GPU-optimized Approaches to Molecular Docking-based Virtual Screening in Drug Discovery: A Comparative Analysis
Source: arXiv:2209.05069 source file (2022-09-12)
Supplement: Supplementary file 1 [file appendix.tex]

\begin{table*}[t]
\centering
\begin{tabular}{|ll|}
  \hline
  Derived Metric & Metrics (\texttt{ncu}) \\
  \hline
  \multirow{2}{*}{Timing} & \texttt{sm\_\_cycles\_elapsed.avg} \\
                          & \texttt{sm\_\_cycles\_elapsed.avg.per\_second} \\
  \hline
  \multirow{10}{*}{FLOP} & \texttt{sm\_\_sass\_thread\_inst\_executed\_op\_dfma\_pred\_on.sum} \\
                         & \texttt{sm\_\_sass\_thread\_inst\_executed\_op\_dmul\_pred\_on.sum} \\
                         & \texttt{sm\_\_sass\_thread\_inst\_executed\_op\_dadd\_pred\_on.sum} \\
                         & \texttt{sm\_\_sass\_thread\_inst\_executed\_op\_ffma\_pred\_on.sum} \\
                         & \texttt{sm\_\_sass\_thread\_inst\_executed\_op\_fmul\_pred\_on.sum} \\
                         & \texttt{sm\_\_sass\_thread\_inst\_executed\_op\_fadd\_pred\_on.sum} \\
                         & \texttt{sm\_\_sass\_thread\_inst\_executed\_op\_hfma\_pred\_on.sum} \\
                         & \texttt{sm\_\_sass\_thread\_inst\_executed\_op\_hmul\_pred\_on.sum} \\
                         & \texttt{sm\_\_sass\_thread\_inst\_executed\_op\_hadd\_pred\_on.sum} \\
                         & \texttt{sm\_\_inst\_executed\_pipe\_tensor.sum} \\
  \hline
  Thread Instructions & $\texttt{smsp\_\_thread\_inst\_executed.sum} / 32$ \\
  \hline
  \multirow{2}{*}{L1 Global Transactions} & \texttt{l1tex\_\_t\_sectors\_pipe\_lsu\_mem\_global\_op\_ld.sum} \\
                                          & \texttt{l1tex\_\_t\_sectors\_pipe\_lsu\_mem\_global\_op\_st.sum} \\
  \hline
  \multirow{2}{*}{L1 Shared Transactions} & \texttt{l1tex\_\_data\_pipe\_lsu\_wavefronts\_mem\_shared\_op\_ld.sum} \\
                                          & \texttt{l1tex\_\_data\_pipe\_lsu\_wavefronts\_mem\_shared\_op\_st.sum} \\
  \hline
  \multirow{4}{*}{L2 Transactions} & \texttt{lts\_\_t\_sectors\_op\_read.sum} \\
                                   & \texttt{lts\_\_t\_sectors\_op\_atom.sum} \\
                                   & \texttt{lts\_\_t\_sectors\_op\_red.sum} \\
                                   & \texttt{lts\_\_t\_sectors\_op\_write.sum} \\
  \hline
  \multirow{2}{*}{DRAM Transactions} & \texttt{dram\_\_sectors\_read.sum} \\
                                     & \texttt{dram\_\_sectors\_write.sum} \\
  \hline
  Warp Instructions & \texttt{smsp\_\_inst\_executed.sum} \\
  \hline
  Warp global loads/stores & \texttt{smsp\_\_inst\_executed\_op\_global\_ld.sum} \\
  \hline
  \multirow{2}{*}{Warp shared loads/stores} & \texttt{smsp\_\_inst\_executed\_op\_shared\_ld.sum} \\
                                            & \texttt{smsp\_\_inst\_executed\_op\_shared\_st.sum} \\
  \hline
  DRAM bytes & \texttt{dram\_\_bytes.sum} \\
  \hline
  L2 bytes & \texttt{lts\_\_t\_bytes.sum} \\
  \hline
  L1 bytes & \texttt{l1tex\_\_t\_bytes.sum} \\
  \hline
  Instruction mix: integer & \texttt{sm\_\_sass\_thread\_inst\_executed\_op\_integer\_pred\_on.sum} \\
  \hline
  Instruction mix: control flow & \texttt{sm\_\_sass\_thread\_inst\_executed\_op\_control\_pred\_on.sum} \\
  \hline
  Instruction mix: inter-thread communication & \texttt{sm\_\_sass\_thread\_inst\_executed\_op\_inter\_thread\_communication\_pred\_on.sum} \\
  \hline
  Instruction mix: memory & \texttt{sm\_\_sass\_thread\_inst\_executed\_op\_memory\_pred\_on.sum} \\
  \hline
  \multirow{3}{*}{Instruction mix: miscellanea} & \texttt{sm\_\_sass\_thread\_inst\_executed\_op\_bit\_pred\_on.sum} \\
                                                & \texttt{sm\_\_sass\_thread\_inst\_executed\_op\_conversion\_pred\_on.sum} \\
                                                & \texttt{sm\_\_sass\_thread\_inst\_executed\_op\_misc\_pred\_on.sum} \\
  \hline
\end{tabular}
\caption{Metrics for the Instruction Roofline Model and Instruction Mix analysis.}
\label{table:metrics}
\end{table*}
Table~\ref{table:metrics} lists the \texttt{ncu} metrics used to measure instructions and data operations on the GPU cores. Translation from the \textit{legacy} \texttt{nvprof} metrics used in~\cite{ding2019instruction} and their \texttt{ncu} counterparts used in this work has been carried out according to~\cite{nvidia2022nsightcli}.
